# Supplementary material for: Competing charge transfer and screening effects in two-dimensional ferroelectric capacitors
Source: arXiv:2311.08187 source file (2023-11-16)
Supplement: Supplementary file 1 [file Supplementary_Material.pdf]

# Competing charge transfer and screening effects in two-dimensional ferroelectric capacitors

Jiawei Huang<sup>†,1</sup> Changming Ke<sup>†,1</sup> Zhuang Qian,<sup>1</sup> and Shi Liu<sup>1,\*</sup>

<sup>1</sup>*Key Laboratory for Quantum Materials of Zhejiang Province,  
Department of Physics, School of Science,  
Westlake University, Hangzhou, Zhejiang 310030, China*

## I. 2D METALLIC MATERIALS AS ELECTRODES

We select 2D metallic materials with lattice constants close to the ground-state values of  $\alpha$ -In<sub>2</sub>Se<sub>3</sub> as electrodes. A total of 18 electrodes, with work functions ranging from 2 to 10 eV, are investigated. The work functions of these electrodes are listed in Table. S1. The atomic positions of electrodes are fully optimized with the in-plane lattice constants fixed to the ground-state value of monolayer  $\alpha$ -In<sub>2</sub>Se<sub>3</sub>. The work functions are then calculated based on the optimized structures. Specifically, Ti<sub>2</sub>I<sub>2</sub> ( $W_M=3.28$  eV) is used to gauge the impact of charge transfer on ferroelectric stability in the low work function region, as shown in Fig. 3a of the main text.

TABLE S1. Work functions (in eV) of 2D electrodes.

| Metal | Ti <sub>2</sub> I <sub>2</sub> | Nb <sub>2</sub> Cl <sub>2</sub> | Ru <sub>2</sub> Te <sub>2</sub> | Ir <sub>2</sub> Te <sub>2</sub> | W <sub>2</sub> Te <sub>2</sub> | Sb <sub>2</sub> Te <sub>2</sub> | Fe <sub>2</sub> Te <sub>2</sub> | Ni <sub>2</sub> Te <sub>2</sub> | Rh <sub>2</sub> Se <sub>2</sub> |
|-------|--------------------------------|---------------------------------|---------------------------------|---------------------------------|--------------------------------|---------------------------------|---------------------------------|---------------------------------|---------------------------------|
| $W_M$ | 3.28                           | 3.48                            | 3.77                            | 3.80                            | 3.81                           | 4.06                            | 4.20                            | 4.51                            | 4.59                            |
| Metal | ZrTeSe                         | Au <sub>2</sub> Se <sub>2</sub> | Au <sub>2</sub> S <sub>2</sub>  | BiSe <sub>2</sub>               | Tl <sub>2</sub> S <sub>2</sub> | AgBr <sub>2</sub>               | HgO <sub>2</sub>                | AgCl <sub>2</sub>               | AgF <sub>2</sub>                |
| $W_M$ | 4.99                           | 5.43                            | 5.84                            | 5.98                            | 6.19                           | 6.82                            | 7.46                            | 7.52                            | 8.39                            |

## II. SWITCHING BARRIERS IN CuInP<sub>2</sub>S<sub>6</sub> AND SnTe

The switching energy barriers in freestanding monolayer CuInP<sub>2</sub>S<sub>6</sub> (CIPS) and SnTe, as well as in capacitors consisting of electrodes of low work function (LW) and high work function (HW), respectively, are analyzed. As illustrated in Fig. S1, the atomic displacements of Cu atoms ( $u_{Cu}$ ) and Te atoms ( $u_{Te}$ ) are used to gauge the polarization switching process. The switching barriers are obtained by manually varying the Cu/Te atomic displacements from the nonpolar state to the polar state. For these 2D ferroelectric-based capacitors, the interlayer distance between ferroelectric layer and electrode is fixed at 3 Å, typical of van der Waals (vdW) interaction range. The calculated work function of freestanding monolayer CIPS and SnTe are 5.27 eV and 3.90 eV, respectively. To reduce the lattice mismatch, we choose Zr<sub>2</sub>Cl<sub>2</sub> ( $W_M=3.75$  eV) as the LW electrode and Ru<sub>2</sub>F<sub>2</sub> ( $W_M=8.24$  eV) as the HW electrode for CIPS; and Sc<sub>2</sub>O<sub>2</sub> ( $W_M=3.33$  eV) as the LW electrode and Bi<sub>2</sub>Cl<sub>2</sub> ( $W_M=6.24$

\* liushi@westlake.edu.cn

eV) as the HW electrode for SnTe. The calculated switching barriers are listed in Table. S2. Notably, both LW and HW electrodes will reduce the switching barriers in CIPS. In comparison, for SnTe, the ferroelectricity is enhanced by the LW electrodes, but suppressed when encapsulated by HW electrodes.

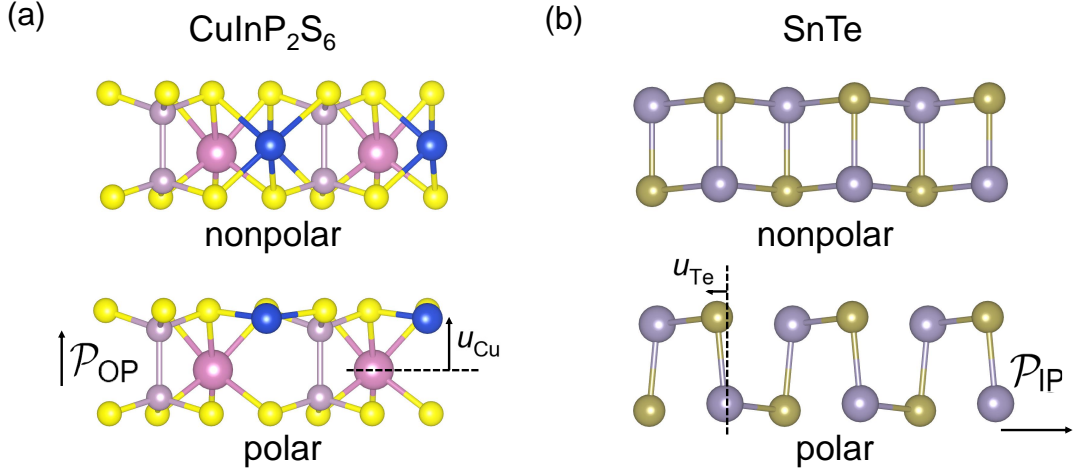

FIG. S1. Nonpolar and polar structures of (a) CIPS and (b) SnTe. The atomic displacement of Cu and Te atom are denoted as  $u_{\text{Cu}}$  and  $u_{\text{Te}}$ , respectively.

TABLE S2. Switching energy barriers in CIPS and SnTe under both open-circuit (without electrodes) and short-circuit (with electrodes) electrical boundary conditions.

|          | LW electrodes                           | HW electrodes                           | without electrodes |
|----------|-----------------------------------------|-----------------------------------------|--------------------|
| CIPS     | 0.458                                   | 0.285                                   | 0.494              |
| (in eV)  | ( $W_{\text{Zr}_2\text{Cl}_2}=3.75$ eV) | ( $W_{\text{Ru}_2\text{F}_2}=8.24$ eV)  | -                  |
| SnTe     | 19.5                                    | -                                       | 1.6                |
| (in meV) | ( $W_{\text{Sc}_2\text{O}_2}=3.33$ eV)  | ( $W_{\text{Bi}_2\text{Cl}_2}=6.24$ eV) | -                  |

### III. CHARGE ANALYSIS OF 2D FERROELECTRIC CAPACITORS

We use the Bader charge analysis to measure the charge transfer between the buffer layer (BL) and the adjacent electrode. It is noted that atoms in the monolayer  $\beta\text{-In}_2\text{Se}_3$  are manually fixed when  $n \geq 3$  since they spontaneously transform into the  $\beta'$  phase during the

relaxation if not. As the thickness of the ferroelectric layer increases, the charge transfer between the top electrode and monolayer  $\beta$ -In<sub>2</sub>Se<sub>3</sub> decreases from 0.122  $e$  to 0.089  $e$ , and the total charge accepted by monolayer  $\beta$ -In<sub>2</sub>Se<sub>3</sub> also decreases from 0.178  $e$  to 0.122  $e$ . According to the quadratic relationship between  $E_b$  and  $Q$  presented in Fig. 2c of the main text, the reduced binding affinity can no longer stabilize  $\beta$ -In<sub>2</sub>Se<sub>3</sub>, thus leading to the  $\beta \rightarrow \beta'$  phase transition.

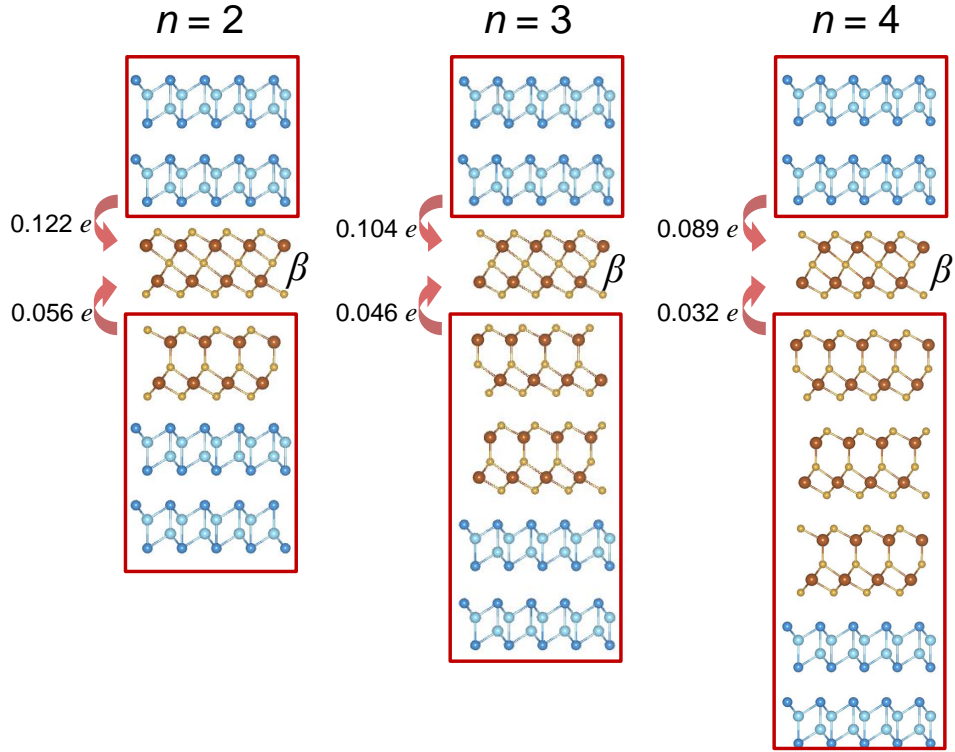

FIG. S2. Evolution of interfacial charge transfer to the buffer layer ( $\beta$ -In<sub>2</sub>Se<sub>3</sub>) in capacitors with increasing thickness of ferroelectric layers.
